# Supplementary material for: What is Point Supervision Worth in Video Instance Segmentation?
Source: arXiv:2404.01990 source file (2024-04-01)
Supplement: Supplementary file 1 [file supp.tex]

\section*{A. Implementation Details of Sampling Points by Distance Transform}
\label{sec:supp_A}
We provide implementation details of distance transform for sampling positive and negative points, respectively. Distance transform is an operator applied to binary images. The resulting distance map is a gray level image that looks similar to the input binary image, except that the gray level intensities of points inside foreground regions are changed to show the distance to the closest boundary from each point. 

We first explain how we sample positive points via distance transform in detail. Given a binary ground truth object mask, we generate its distance map by applying distance transform directly to the foreground mask. The resulting distance map has zero values outside the foreground region and positive values inside the foreground region, indicating the euclidean distance to the closest boundary for each point. We then normalize the distance values to obtain the distribution used for sampling points, and randomly sample positive points given the resulting distribution.

We sample negative points via distance transform in a similar way, as shown in Figure~\ref{fig:supp_sample_neg}. We first apply distance transform to the inverse of the foreground mask (\ie background region has value one while the foreground region has value zero). We then threshold the resulting distance map with a fixed pixel values (\eg 50) and only keep the pixels whose distance is within the distance threshold. Finally, we sample negative points randomly inside the kept pixels. By setting different threshold, we can control how far away the negative points are sampled.

\begin{table*}[t]
	\centering
	\footnotesize
	
    \renewcommand{\tabcolsep}{2pt}
	
	\resizebox{1.0\textwidth}{!}{
		%\begin{tabular}{llllllllllllllllllllll}
  \begin{tabular}{lccccccccccccccccccccc}
			\toprule
			Methods  & person & panda &lizard & parrot &skateboard& sedan & ape &dog& snake&monkey&hand&rabbit&duck&cat&cow&fish&train&horse&turtle&bear&\textbf{mAP}  \\  
            MinVIS~\cite{huang2022minvis} &53.3 & 71.8 & 83.5 & 79.6 & 21.0 & 61.5 & 47.2 & 55.6 & 47.0 & 35.4 & 59.8 & 93.4 &54.9 & 77.3 & 66.1 & 24.0 & 58.7 & 47.1 & 57.3 & 62.3 & -\\
		\textbf{PointVIS} & 47.7 & 56.6& 55.6& 68.2 & 11.9& 58.5 & 38.2 & 50.0 & 37.3 & 23.8 & 44.7 & 89.3 & 48.2 & 58.4 & 68.4 & 2.3 &66.7 & 47.5 & 57.3 & 63.3 &  - \\

  \midrule
  	Methods  & motorbike &giraffe & leopard &fox & deer & owl & surfboard & airplane & truck & zebra & tiger & elephant & snowboard & boat & shark & mouse & frog & eagle & seal & tennis racket &\textbf{mAP}  \\  
            MinVIS~\cite{huang2022minvis} &  40.9 & 70.5 & 59.0 & 41.9 & 65.6 & 57.2 & 8.4 & 37.2 & 72.4 & 72.2 & 57.6 & 70.6 & 0.2 & 69.0 & 58.5 & 60.4 & 3.7 & 84.4 & 56.4 &37.1&55.3\\
		\textbf{PointVIS} & 36.7 & 66.2& 35.0 & 39.2 & 55.3 & 48.7 & 0.0& 44.7 & 64.6 &55.9 &48.8 & 58.5 & 5.5 & 56.6&23.9 & 35.7 & 12.2 & 72.2 &51.4 &33.7 &46.0\\
			\bottomrule
	\end{tabular}}
        \caption{\textbf{Per-class and overall mAP results for MinVIS~\cite{huang2022minvis} and PointVIS (P1, w/o self-training) on Youtube-VIS 2019 val-dev}. All models here use Swin-B as the backbone.}
	\label{tab:per-category}
\end{table*}

%%%%%%%%%%%%%%%%%%%%%%Sampling method Ablation
\section*{B. More Ablation on Point Selection Bias}
\label{sec:supp_B}
To further investigate the point selection bias, we report ablation results with additional negative point sampling methods in Table~\ref{tab:supp_bias}. We additionally sample negative points by randomly sampling from the region outside the ground truth mask (Random (Out-mask)) or by negative distance transform (Random (Distance Transform)). We observe that different negative points sampling methods achieve comparable results. This result show that our method is generally robust to the negative point location, thanks to our point-based matcher that incorporates annotation-free negative cues.

\begin{figure}[b]
  \centering
  \includegraphics[width=1.0\linewidth]{./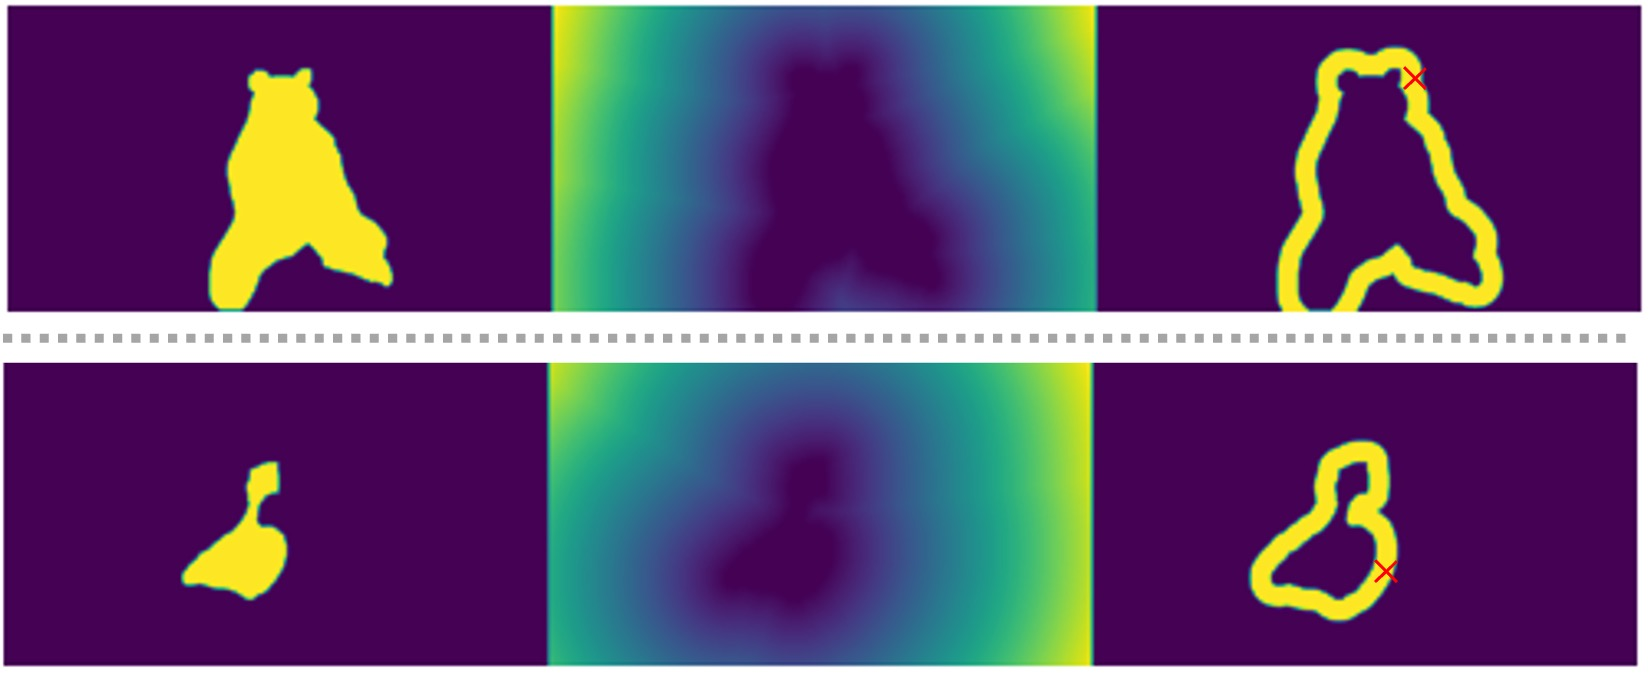}
    \caption{\textbf{Visualization of sampling negative points with distance transform.} From left to right is the ground truth foreground mask, heatmap of the distance transform of the ground truth background mask (the lighter the larger distance), region left for negative points sampling after thresholding a distance of 50 pixels. Red cross indicates the position of the sampled negative points.}

  \label{fig:supp_sample_neg}
\end{figure}

\begin{table}[t]
\footnotesize

\renewcommand{\tabcolsep}{6pt}
\centering
	\resizebox{1.0\linewidth}{!}{
		\begin{tabular}{@{}llll@{}}
			\toprule                
			Model ID & Sampling method for Pos&Sampling method for Neg&AP (\%) \\
			\midrule
			PointVIS (P1) &Random&-& 46.0   \\
			PointVIS (P1) &Distance Transform&-  & 47.1  \\
			\midrule
		    PointVIS (P1N1) &Random&Random (In-box)& 48.6   \\
			PointVIS (P1N1) &Random&Random (Out-box-but-in-200$\%$-box)  & 48.0  \\
			PointVIS (P1N1) &Random&Random (Out-mask)& 48.5   \\
			
		%(threshold 50.0 pixels)
			PointVIS (P1N1) &Random&Random (Distance Transform)   & 48.8  \\
			\bottomrule
		\end{tabular}
	}
\caption{\textbf{Analysis of point selection bias on YouTube-VIS 2019~\cite{yang2019video} val-dev.}}
\label{tab:supp_bias}
\end{table}

% \begin{figure}[b]
%   \centering
%   \includegraphics[width=1.0\linewidth]{submission/figures_supp/vis_supp_dist-tnf-pos.jpg}
%     \caption{\textbf{Sampling positive points w/ distance transform.}}

%   \label{fig:vis_sample_pos}
% \end{figure}

%%%%%%%%%%%%%%%%%%%%%%%%%%%%%%%%%%%%%%%%%%%%%%%%%%%%%%%

\section*{C. More Analysis of Pretrained models.}
\label{sec:supp_C}
As we focus on reducing video annotations, we therefore follow the existing work~\cite{wang2021end,yang2021crossover,huang2022minvis} that use pretrained instance segmentation models. To further study the impact of pretrained models, we additionally report PointVIS (P1) results on YouTube-VIS 2019 val-dev by using different pretrained backbones to generate pseudo-labels while using the same backbone to finetune videos as shown in Table~\ref{tab:R2_diff_backbone}, and pretraining on COCO with less frames as shown in Table~\ref{tab:R2_coco_subsample}. PointVIS achieves competitive results with varying quality of pretrained models.

\begin{table}[t]
\footnotesize
    \begin{minipage}{.23\textwidth}
    \centering
    \vspace{-0.5em}
    \resizebox{1.0\linewidth}{!}{
    \begin{tabular}{@{}llc@{}}
    \toprule
        \makecell{Image \\Pretraining} & \makecell{Video\\Finetuning}& \makecell{mAP \\ \%}\\
        \midrule
         R101&Swin-B & 42.5 \\
      Swin-B&Swin-B & 46.0 \\
         \bottomrule
    \end{tabular}
    }
     \caption{\textbf{Pretraining  with Different models.}}
    \label{tab:R2_diff_backbone}
    \end{minipage}
    \hfill
    \begin{minipage}{.24\textwidth}
    \renewcommand{\tabcolsep}{1pt}
    
    \centering
    
    \vspace{-0.3em}
    \resizebox{1.0\linewidth}{!}{
    \begin{tabular}{@{}l l l l l @{}}
    \toprule
     COCO Frames & 1\%  & 5\% & 10\% & 100\%\\
        \midrule
        mAP \% & 41.2 & 43.0 & 45.3  & 46.0\\
   
         \bottomrule
    \end{tabular}
    }
     \vspace{1.0em}
    \caption{\textbf{Pretraining with different number of COCO images.}} 
      \label{tab:R2_coco_subsample}
    \end{minipage}
  
\end{table}

%%%%%%%%%%%%%%%%%%%%%%%%%%%%%%%%%%%%%%%%%%%%%%%%%%%%%%%%%%%

\section*{D. More Analysis of Generality}
\label{sec:supp_D}
 To validate the generality, we additionally report mAP of 19 seen and 21 unseen categories (Table~\ref{tab:R2_unseen}) on YouTube-VIS 2019 val-dev. PointVIS achieves good results on unseen categories with point labels. We also report per-category results in Table~\ref{tab:per-category} for reference.

\section*{E. Upperbound of More Points}
\label{sec:supp_E}
Treating the ground truth mask as a set of points, we implemented an unpperbound model of our PointVIS (Table~\ref{tab:R2_more_pts}). The upperbound performance (50.0\% mAP) does not match the fully-supervised counterpart (55.3\% mAP), as it is bounded by proposals quality. Our PointVIS instead could approach this upperbound with very little point supervision (saturated at 49.5\% mAP w/ P10N10). 

 \begin{table}[t]
\footnotesize
    \begin{minipage}{.27\textwidth}
    \centering

    %\vspace{-0.9em}
    \renewcommand{\tabcolsep}{0.7em}
     \resizebox{1.0\linewidth}{!}{
    \begin{tabular}{@{}l l l l l @{}}
    \toprule
     Model & Sup. &  \makecell{mAP \\(seen)} & \makecell{mAP \\(unseen)}  & \makecell{mAP \\(all)} \\
        \midrule
        MinVIS~\cite{huang2022minvis} &  $\mathcal{M}$    & 51.6\%  & 58.0\% & 55.3\% \\
        \midrule
        PointVIS (ours) & $\mathcal{P}_1$ & 47.1\% & 44.9\% & 46.0\% \\
         \bottomrule
    \end{tabular}
    }
    \caption{\textbf{ Unseen categories evaluation on YouTube-VIS 2019 val-dev.}}
    \label{tab:R2_unseen}
    \end{minipage}
    \hfill
    \begin{minipage}{.20\textwidth}
    \renewcommand{\tabcolsep}{1pt}
    
    \centering
    %\vspace{-1.2em}
    \renewcommand{\tabcolsep}{0.7em}
     \resizebox{1.0\linewidth}{!}{
    \begin{tabular}{@{}l l   l @{}}
    \toprule
     Model & Matching  & mAP \\
        \midrule
        MinVIS~\cite{huang2022minvis} &  /    & 55.3\% \\
        \midrule
        % PointVIS (ours) & P1 & Pseudo Mask & 49.4\% & 46.0\% \\
        PointVIS (ours) & P10N10 & 49.5\% \\
        PointVIS (upperbound) & GT Mask & 50.0\% \\
         \bottomrule
    \end{tabular}
    }
    \vspace{+1.5mm}
    \caption{\textbf{ More points oracle on YouTube-VIS 2019 val-dev.}}
    \label{tab:R2_more_pts}
    \end{minipage}
\end{table}

%%%%%%%%%%%%%%%%%%%%%%%%%%%Three benchmarks in one table

\section*{F. More Quantitative Results}
\label{sec:supp_F}
To have a better understanding of our method, we additionally report quantitative performance of our \ours w/o self-training on Youtube-VIS 2019~\cite{yang2019video}, Youtube-VIS 2021~\cite{yang2019video} and OVIS~\cite{qi2021occluded} validation set for reference, as summarized in Table~\ref{tab:supp_main}. High retention rate across three benchmarks indicates the effectiveness of our method.

\begin{table*}[t]
\centering
\resizebox{\textwidth}{!}{
\addtolength{\tabcolsep}{4pt}
\tabfontsize
\begin{tabular}{llllllllll}
\toprule
Method       &Dataset   &Sup. & AP (\%)   & AP$_{50}$ (\%) & AP$_{75}$ (\%) & AR$_1$ (\%) & AR$_{10}$ (\%) \\\midrule
TeViT~\cite{yang2022tevit}           & YouTube-VIS-2019  &$\mathcal{M}$ & 56.8 & 80.6    & 63.1    & 52.0   & 63.3    \\
IDOL~\cite{IDOL}            & YouTube-VIS-2019 &$\mathcal{M}$& 64.3 & 87.5    & 71.0    & 55.6   & 69.1    \\
MinVIS~\cite{huang2022minvis} &YouTube-VIS-2019 &$\mathcal{M}$ & 61.6 & 83.3    & 68.6    & 54.8   & 66.6    \\
\ours (P1)*        & YouTube-VIS-2019  &$\mathcal{P}_1$   & 52.5 (85.2\%) & 74.5 (89.4\%)    & 59.2 (86.3\%)    & 47.2 (86.1\%)  & 61.5 (92.3\%)    \\
\ours (P1)     &YouTube-VIS-2019    & $\mathcal{P}_1$   & 53.9 (87.5\%) & 75.7 (90.9\%)    & 61.8 (90.1\%)    & 47.5 (86.7\%)   & 61.4 (92.2\%)    \\
\ours (P1N1)*      & Swin-L &$\mathcal{P}_2$    & 57.6 (93.5\%) & 79.9 (95.9\%)    & 63.9 (93.1\%)    & 52.2 (95.2\%)   & 62.7 (94.1\%)    \\
\ours (P1N1)     &YouTube-VIS-2019    & $\mathcal{P}_2$   & 59.6 (96.7\%) & 83.3 (100\%)    & 67.1 (97.8\%)    & 52.7 (96.2\%)   & 63.8 (95.8\%)    \\

\midrule
SeqFormer~\cite{wu2021seqformer}       & YouTube-VIS-2021   & $\mathcal{M}$ & 51.8 & 74.6    & 58.2    & 42.8   & 58.1    \\
IDOL~\cite{IDOL}            & YouTube-VIS-2021    & $\mathcal{M}$  & 56.1 & 80.8    & 63.5    & 45.0   & 60.1    \\
MinVIS~\cite{huang2022minvis}   &YouTube-VIS-2021        &$\mathcal{M}$& 55.3 & 76.6    & 62.0    & 45.9   & 60.8    \\
\ours (P1)*            & YouTube-VIS-2021   &$\mathcal{P}_1$  & 46.0 (83.2\%) & 70.3 (91.8\%)    & 50.1 (80.8\%)    & 39.2 (85.4\%)  & 52.9 (87.0\%)    \\
\ours(P1)     &YouTube-VIS-2021       & $\mathcal{P}_1$  & 46.3 (83.7\%) & 70.5 (92.0\%)    & 51.1 (82.4\%)    & 37.7 (82.1\%)   & 52.9 (87.0\%)    \\
\ours (P1N1)*            & YouTube-VIS-2021   &$\mathcal{P}_2$ & 47.6 (86.1\%) & 72.2 (94.2\%)    & 53.0 (85.5\%)    & 40.7 (88.7\%)   & 53.9 (88.7\%)    \\
\ours(P1N1)    &YouTube-VIS-2021     &$\mathcal{P}_2$  & 48.5 (87.7\%) & 73.0 (95.3\%)    & 54.4 (87.7\%)   & 41.7 (90.8\%)   & 54.1 (89.0\%)    \\

\midrule
 
MaskTrack~\cite{li2021limited} & Occluded VIS         &$\mathcal{M}$  &28.9 &56.3& 26.8& 13.5& 34.0 \\
IDOL~\cite{IDOL} & Occluded VIS         &$\mathcal{M}$  &42.6&	65.7&	45.2&			17.9&		49.6 \\
MinVIS~\cite{huang2022minvis}         & Occluded VIS         &$\mathcal{M}$   & 39.4 & 61.5  & 41.3      & 18.1   & 43.3      \\
\ours (P1)*                 &  Occluded VIS &$\mathcal{P}_1$ & 27.0 (68.5\%) & 48.5 (78.9\%) & 25.2 (61.0\%)      & 13.8 (76.2\%)   & 32.1 (74.1\%)      \\
\ours (P1)                 &  Occluded VIS   &$\mathcal{P}_1$ & 28.6 (72.6\%) & 49.6 (80.7\%) & 27.5 (66.6\%)      & 15.0 (82.9\%)   & 32.8 (75.8\%)      \\
\ours (P1N1)*                 & Occluded VIS &$\mathcal{P}_2$ & 27.4 (69.5\%) & 48.7 (79.2\%) & 25.5 (61.7\%)    & 13.9 (76.8\%)   & 31.5 (72.7\%)     \\
\ours (P1N1)            & Occluded VIS  &$\mathcal{P}_2$ & 28.6 (72.6\%) & 51.2 (83.3\%) & 27.2 (65.9\%)     & 14.7 (81.2\%)  & 32.2 (74.4\%)      \\
\bottomrule
\end{tabular}
}

\caption{\textbf{Full mask ($\mathcal{M}$) vs. our point supervision ($\mathcal{P}$) on validation set of YouTube-VIS 2019~\cite{yang2019video}, YouTube-VIS 2021~\cite{yang2019video}, and OVIS~\cite{qi2021occluded}.} All results below are based on Swin-L backbone. * denotes our PointVIS results w/o self-training.}

% \caption{\textbf{Full mask ($\mathcal{M}$) vs. new point supervision ($\mathcal{P}$) on validation set of YouTube-VIS 2019~\cite{yang2019video}, YouTube-VIS 2021~\cite{yang2019video}, and OVIS~\cite{qi2021occluded}.} All results below are based on Swin-L backbone. Our PointVIS results are with self-training. See text for more details.}
\label{tab:supp_main}
\end{table*}
%%%%%%%%%%%%%%%%%%%%%%%%%%%%%%%%%%%%%%%%%%%%%%%%%%%%%%%%%%

%%%%%%%%%%%%visualization of sampling methods
% \begin{figure}[htbp]
% \begin{minipage}[t]{0.45\linewidth}
%     \includegraphics[width=\linewidth]{submission/figures_supp/vis_supp_dist-tnf-pos.jpg}
%     \caption{caption1}
%     \label{f1}
% \end{minipage}%
%     \hfill%
% \begin{minipage}[t]{0.45\linewidth}
%     \includegraphics[width=\linewidth]{submission/figures_supp/vis_supp_dist-tnf-neg.jpg}
%     \caption{caption2}
%     \label{f2}
% \end{minipage} 
% \end{figure}

%%%%%%%%%%%%%

%%%%%%%%%%%%%%%%%%%visualization of supp three benchmarks
\section*{G. More Qualitative Results}
\label{sec:supp_G}
More qualitative results from the predictions of our \ours on Youtube-VIS 2019~\cite{yang2019video}, Youtube-VIS 2021~\cite{yang2019video} and OVIS~\cite{qi2021occluded} validation set, are shown in Figure~\ref{fig:vis_supp_ytvis19}, ~\ref{fig:vis_supp_ytvis21} and ~\ref{fig:vis_sup_ovis}, respectively.

\begin{figure*}[t]
  \centering
  \includegraphics[width=1.0\linewidth]{./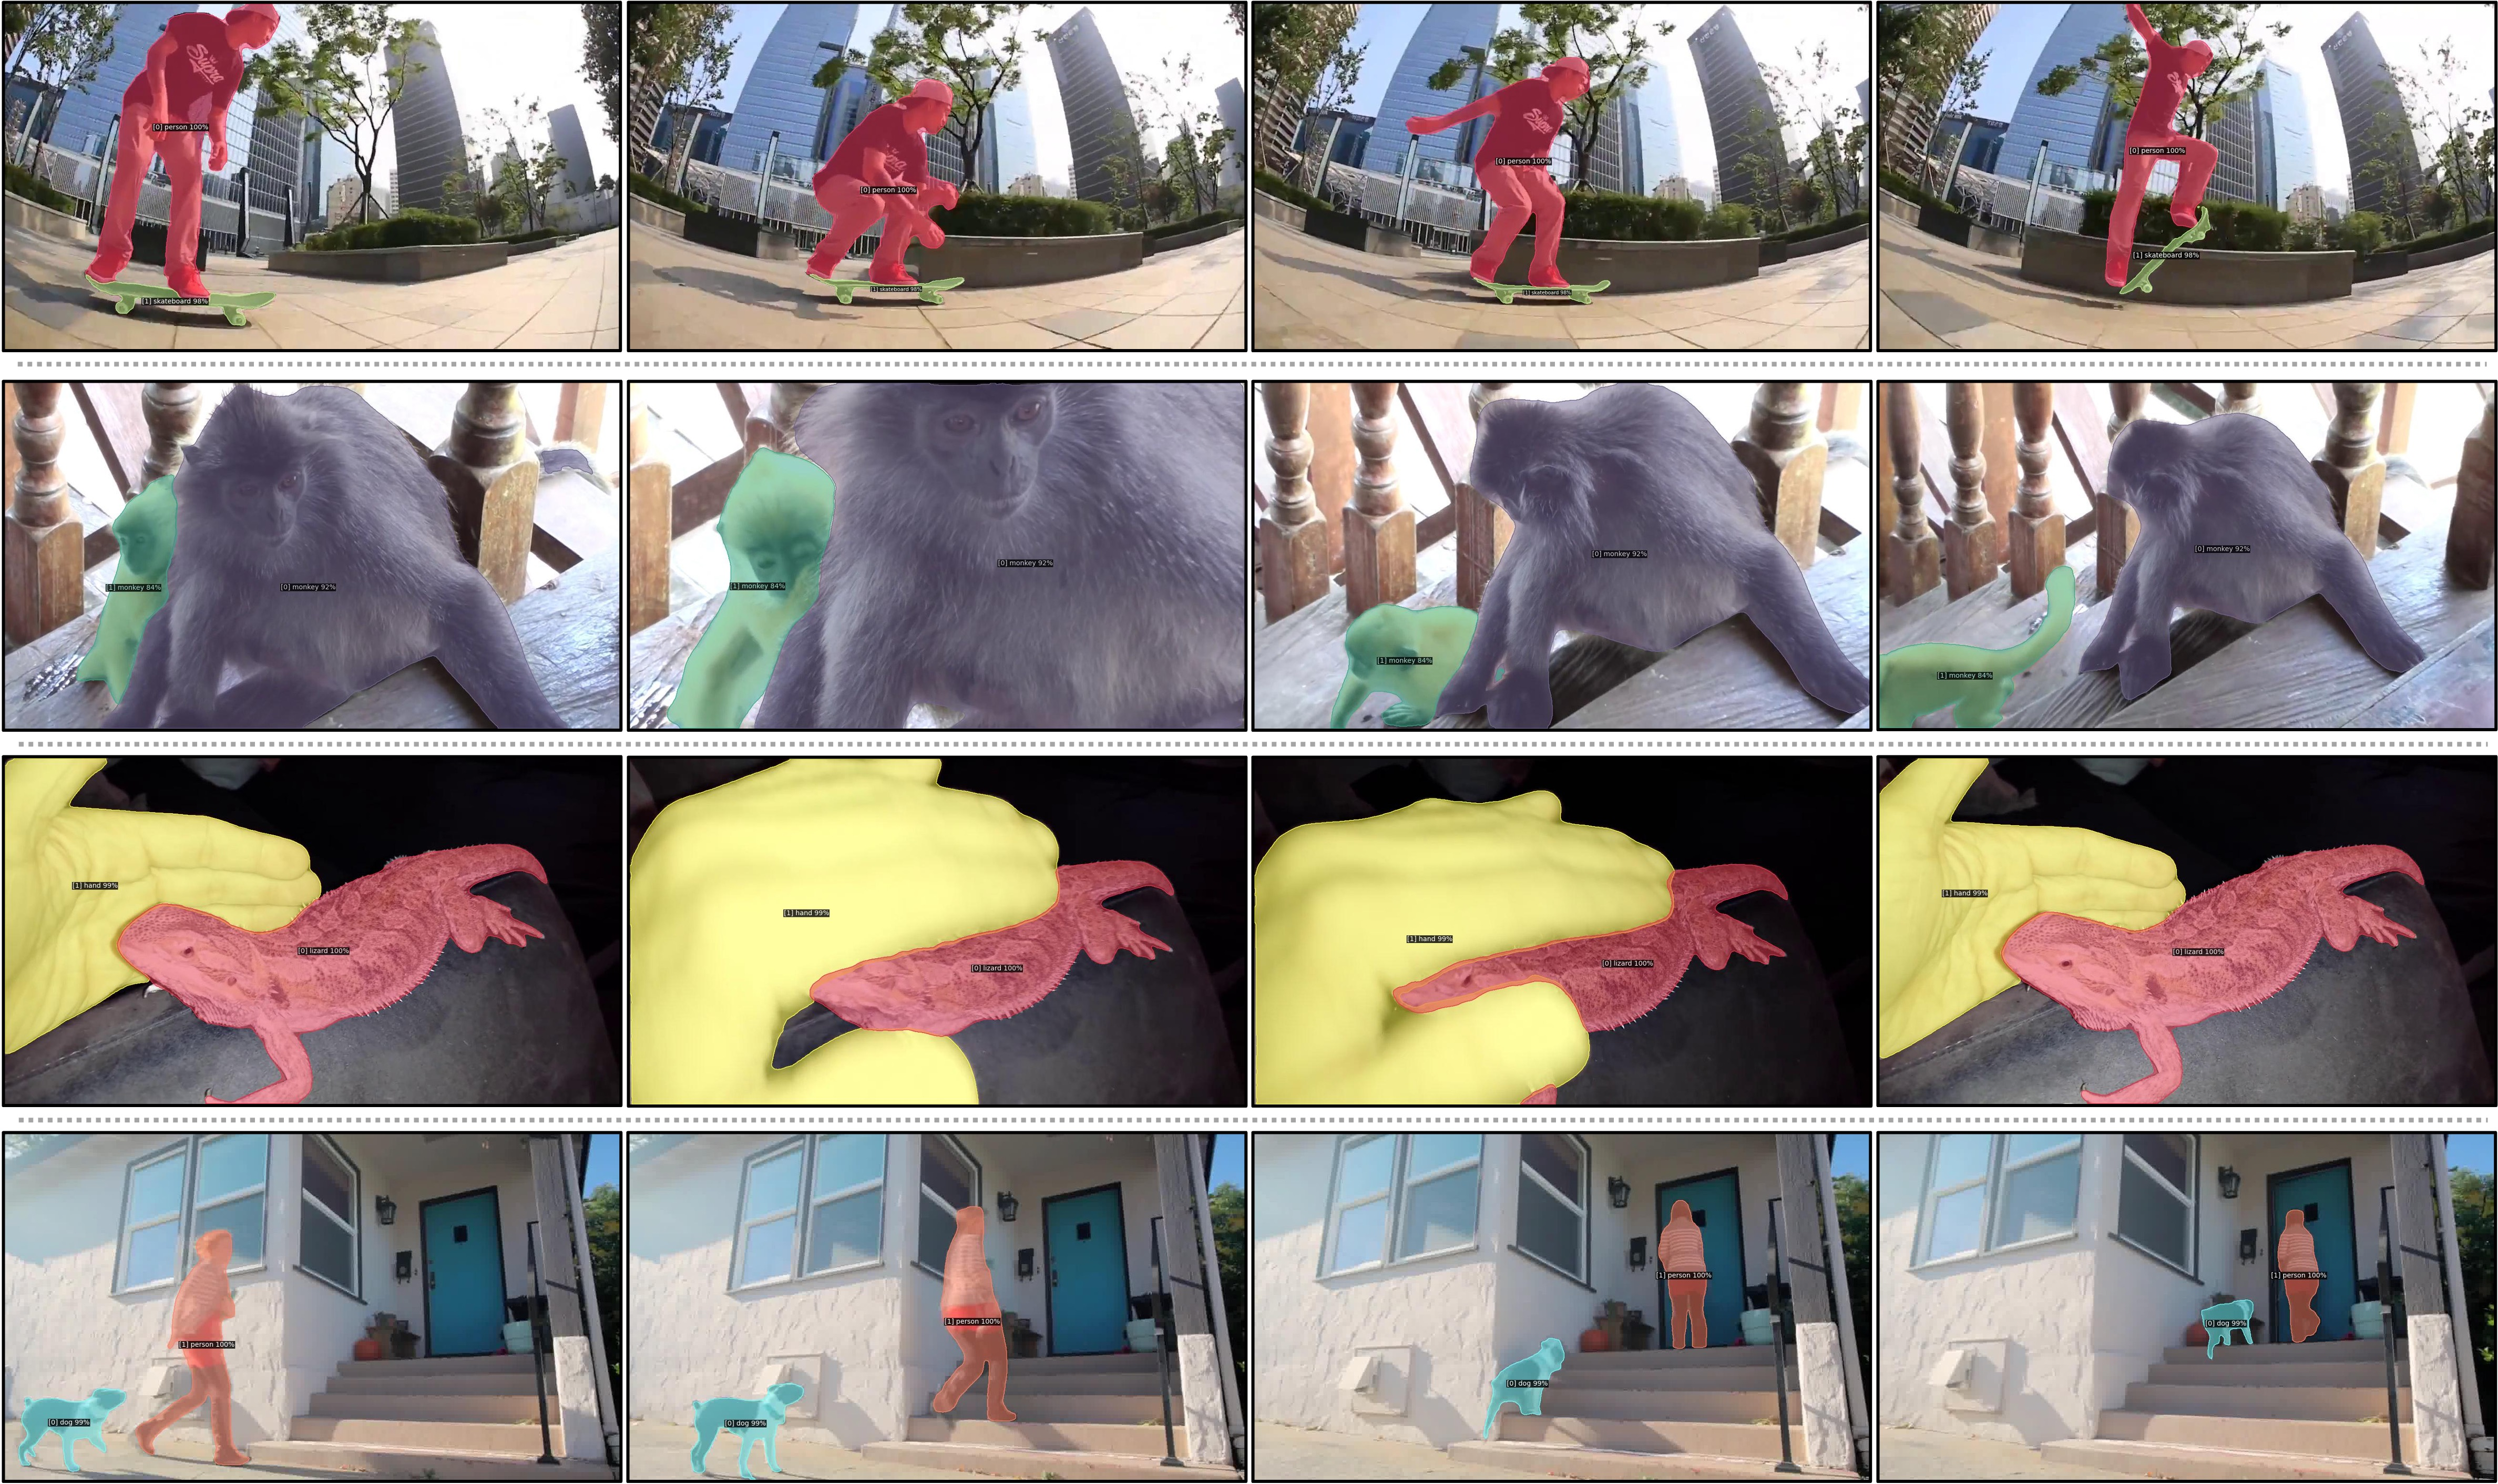}
  \caption{Visualization of predictions from our \ours on Youtube-VIS 2019~\cite{yang2019video} validation set.}
  \label{fig:vis_supp_ytvis19}
\end{figure*}

\begin{figure*}[t]
  \centering
  \includegraphics[width=1.0\linewidth]{./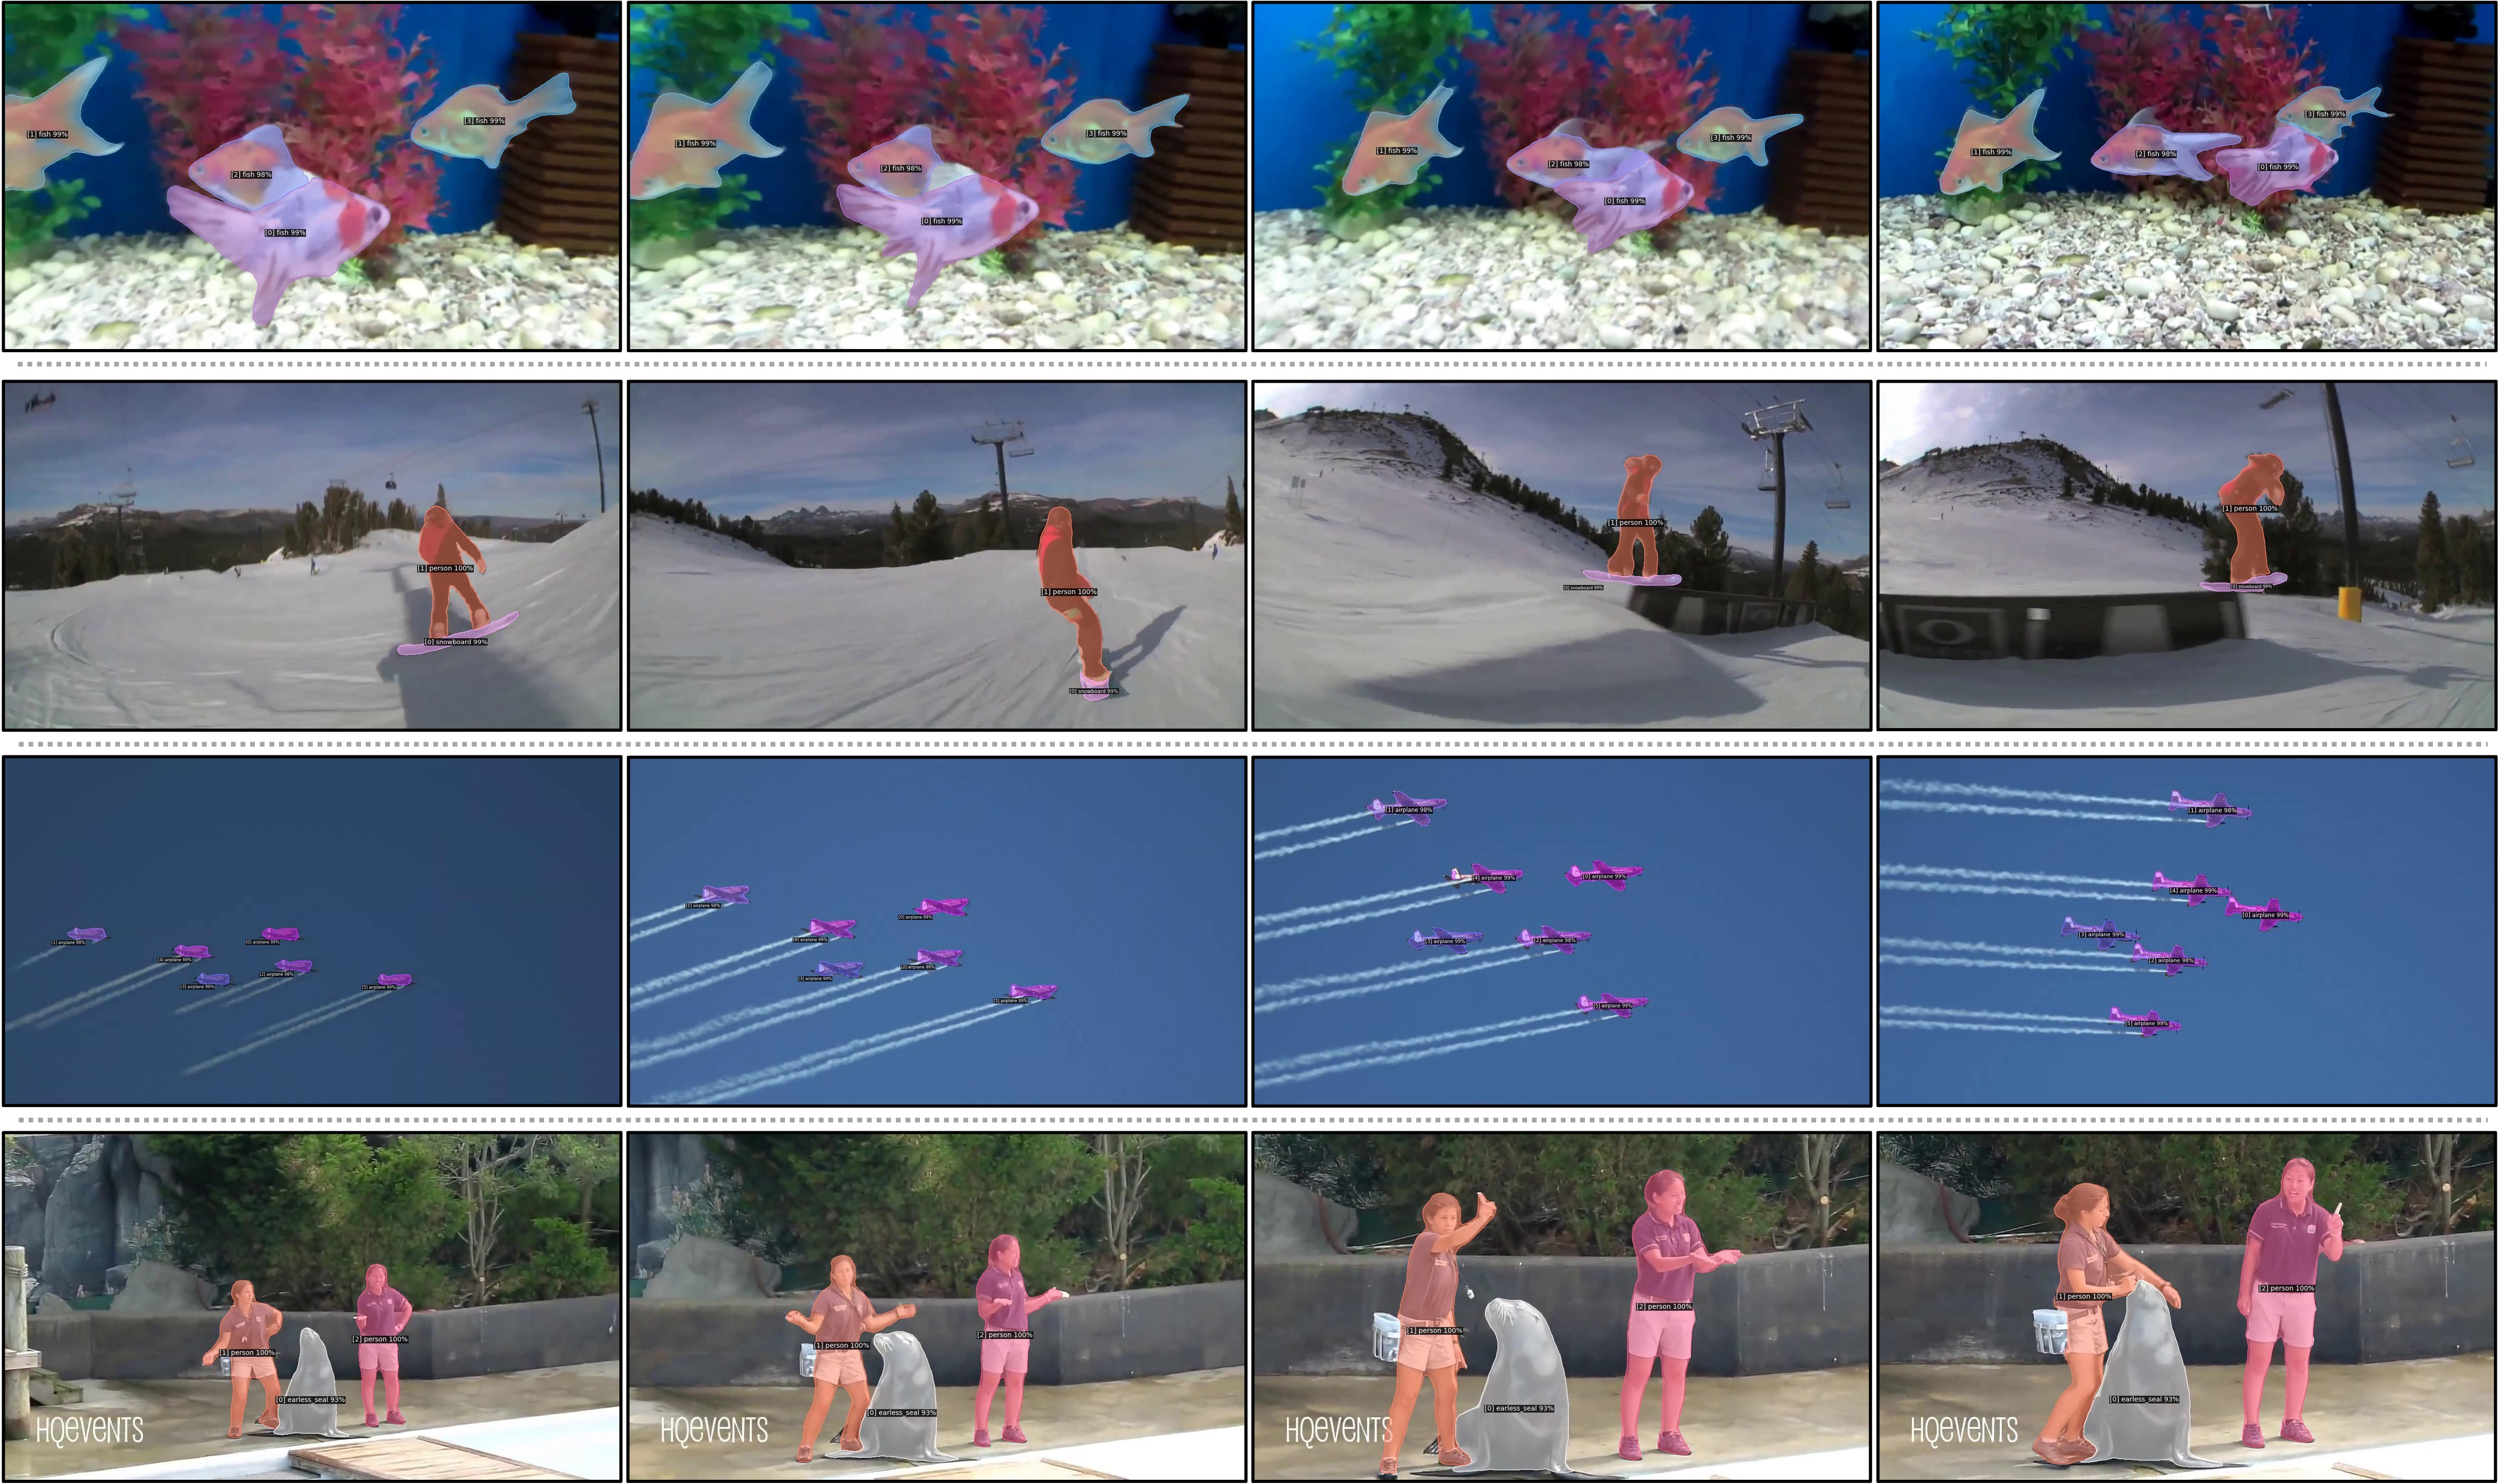}
  \caption{Visualization of predictions from our \ours on Youtube-VIS 2021~\cite{yang2019video} validation set.}
  \label{fig:vis_supp_ytvis21}
\end{figure*}

\begin{figure*}[t]
  \centering
  \includegraphics[width=1.0\linewidth]{./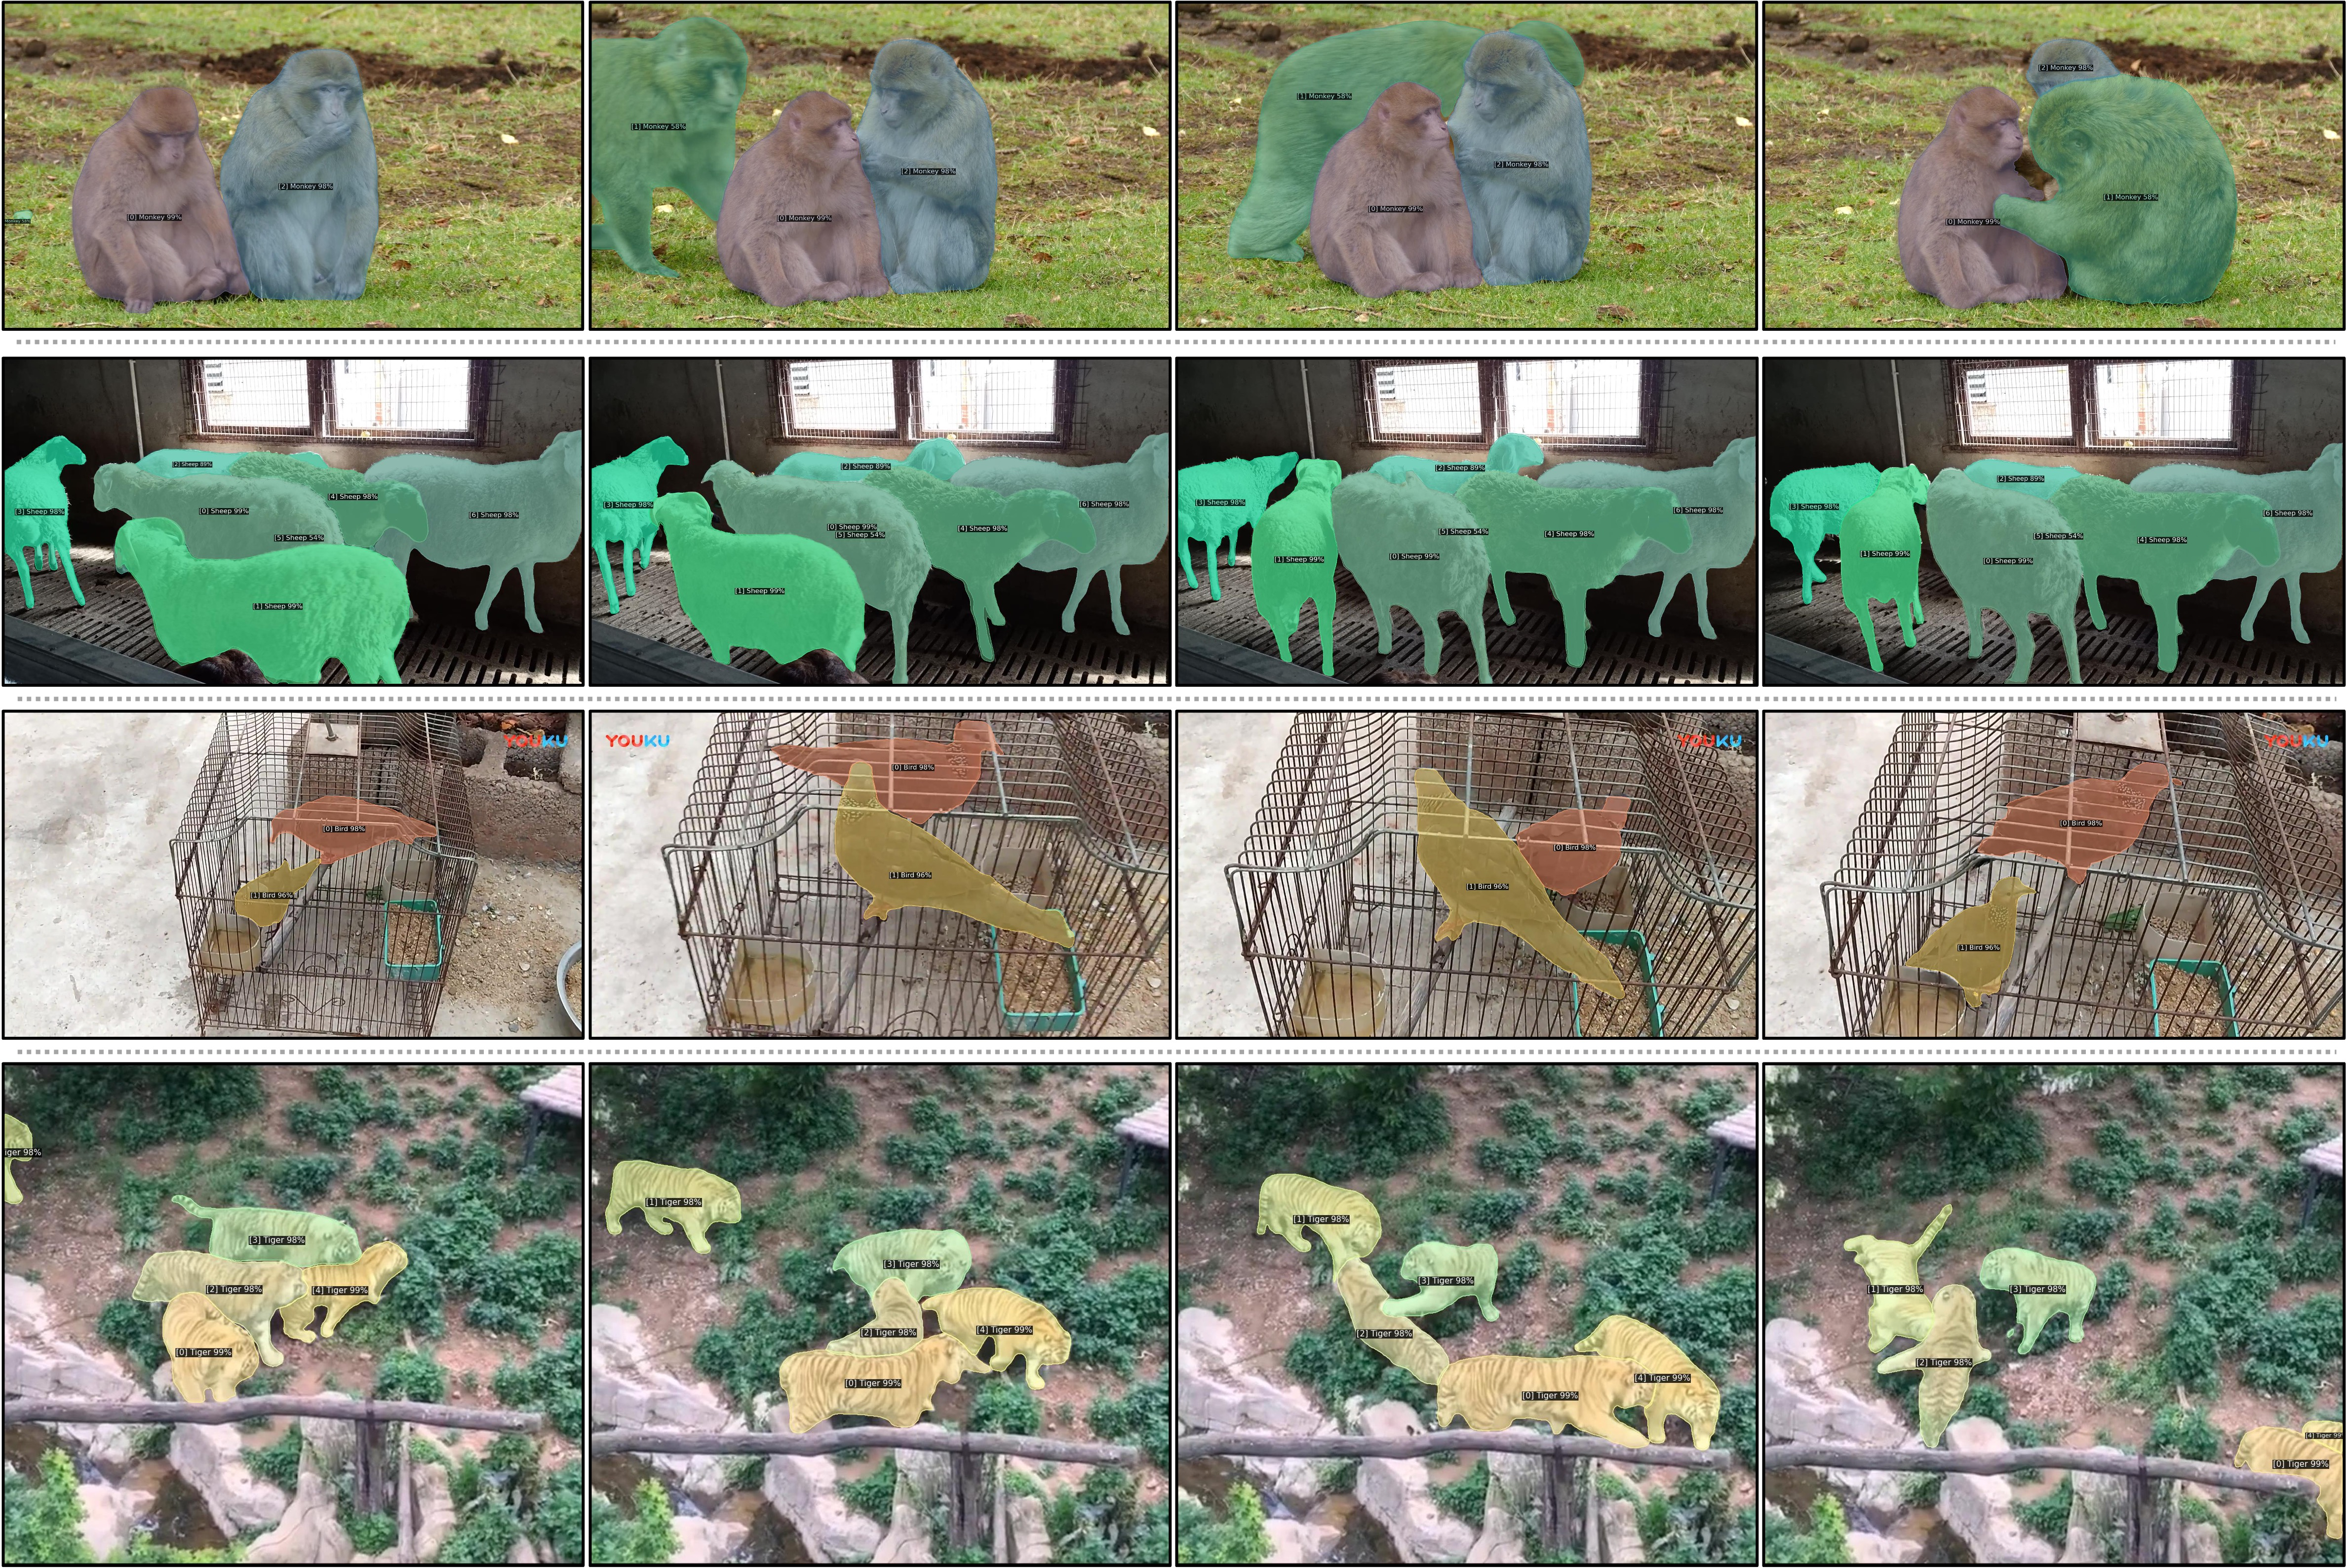}
  \caption{Visualization of predictions from our \ours on OVIS~\cite{qi2021occluded} validation set.}
  \label{fig:vis_sup_ovis}
\end{figure*}

%%%%%%%%%%%%%%%%%%%%%%%%%%%%%%%%%%%%%%%%%%%%%%%
